# Supplementary material for: Origin of reversible photo-induced phase separation in hybrid perovskites
Source: arXiv:1606.07366 ancillary file (2016-06-24)
Supplement: Supplementary file 1 [file Bischak-SI-2016-06-22-forarxiv.pdf]

# Supplementary Materials

## Origin of reversible photo-induced phase separation in hybrid perovskites

Connor G. Bischak, Craig L. Hetherington, Hao Wu, Shaul Aloni, D. Frank Ogletree, David T. Limmer, Naomi S. Ginsberg

correspondence to: nsginsberg@berkeley.edu

**Supplementary Materials contents:**

Materials and Methods
Supplementary Text
Figs. S1 to S13
Captions for Movies S1 to S6

**Other Supplementary Materials for this manuscript includes the following:**

Movies S1 to S6

## Materials and Methods

Perovskite Deposition

$MAPb(Br_xI_{1-x})_3$ was deposited via spin coating at 2000 rpm from 0.55 M solutions containing different ratios of $PbBr_2$ (Aldrich), $CH_3NH_3Br$ (Dyesol) , $PbI_2$ (Aldrich), and $CH_3NH_3I$ (Dyesol) in DMF (Aldrich). For CL and SEM imaging and *in situ* acquisition of PL spectra, films were deposited on Si substrates and annealed in air at 100 °C for 5 min. Films on Si were stored in $N_2$ prior to imaging. For confocal microscopy and PL spectra acquired outside of the SEM chamber, films were deposited on glass cover slips and annealed in air at 100 °C for 5 min. A thin (~0.5-1.0 μm) layer of poly(methyl methacrylate) (PMMA, Aldrich) in anisole (Aldrich) was spun onto the sample to protect them from moisture. All substrates were cleaned prior to perovskite deposition by sonicating in acetone (Aldrich) and isopropyl alcohol (Aldrich) for 5 min each followed by $O_2$ plasma cleaning in a reactive ion etch (RIE) for 5 min. $MAPb(Br_xCl_{1-x})_3$ films were made using an identical procedure, replacing DMF with dimethyl sulfoxide (DMSO), $PbI_2$ with $PbCl_2$ (Aldrich), and $CH_3NH_3I$ with $CH_3NH_3Cl$ (Dyesol).

$CsPb(Br_xI_{1-x})_3$ films were fabricated by making 0.3 M solutions of CsBr (Aldrich)/$PbBr_2$ and CsI (Aldrich)/$PbI_2$ in DMSO and then mixing these solutions in the appropriate ratio. Solutions were stirred for 1 h at 150 °C. Films were deposited on glass cover slips (prepared as described above) by filtering through a 0.2 μm filter and spin coating while keeping the solution at ~150 °C. All films were annealed at 75 °C for 10 min. A thin (~0.5-1.0 μm) layer of PMMA was spun onto the sample to protect them from moisture.

Cathodoluminescence (CL) and Scanning Electron Microscopy (SEM)

Cathodoluminescence (CL) and secondary electron (SE) images were acquired with a modified Zeiss Gemini SUPRA 55 S2 Scanning Electron Microscope (SEM). An aluminum parabolic reflector was positioned above the sample in order to couple a 1.3π sr solid angle of emission into a photomultiplier tube (Hamamatsu, H7421-40) outside of the vacuum chamber. A 405 nm LED (M405L2, Thorlabs) was used for *in situ* illumination and as the excitation source for the collection of PL spectra. All CL images were acquired by first blanking the electron beam, moving to the region of interest, and then recording an image. Light soaking and CL acquisition were alternated to acquire image series. All CL images were acquired with 512 x 512 pixels of a 10 μm x 10 μm field of view, a scan rate of 10 ms/line, a current of 50 pA, and an accelerating voltage of 3.0 kV. A 590 nm longpass filter was used during CL acquisition. Higher resolution SE images were acquired after CL image acquisition with 1024 x 1024 pixels and a scanning rate of 20 ms/line. For CL and PL spectral acquisition, the SEM was fitted with a fiber-coupled QE65PRO spectrometer with a HC1-QE grating (Ocean Optics).

Confocal Microscopy and Photoluminescence (PL) Spectra

Confocal microscopy images were collected with an IX83 inverted microscope (Olympus) using a 40x 0.95 NA objective. Images of the Br-rich and I-rich regions were acquired simultaneously using a 560 nm dichroic filter and grating set to 500-550 nm and 650-700 nm, for the Br-rich and I-rich regions, respectively. All images were acquired with 512 x 512 pixels with a 200 μm x 200 μm field of view and a scan rate of 10 ms/line. For the I-rich cluster stabilization demonstration (Figure S5), light soaking was induced with a

405 nm LED (M405L2, Thorlabs) at 100 mW/cm$^2$, an image was acquired with a 405 nm laser at, a 635 nm laser was positioned in the center of the field of view at 20.0 μW, and after five minutes another image was acquired with the 405 nm laser at 4.0 μW. For the film luminescence patterning demonstration (Figure S6), the film was constantly illuminated with a 660 nm LED (Thorlabs, M660L3) at 450 mW/cm$^2$. A 405 nm laser (350 nW) was used to induce halide phase separation locally for 2 min at each position. To probe the induced pattern, a 405 nm laser (4.0 μW) was used, scanning at 10 ms/line. PL spectra were acquired using a 405 nm LED (M405L2, Thorlabs) as the excitation source and a fiber-coupled QE65PRO spectrometer with a HC1-QE grating (Ocean Optics).

**Theoretical and computational methods**

Intermolecular potential

The model we use to simulate the mixed halide hybrid perovskite borrows significantly from recent work by Mattoni et al. (*1*) and older work by Lewis and Catlow (*2*). Specifically we adopt the mixed Lennard-Jones

$$U(r) = 4\epsilon \left[ \left(\frac{\sigma}{r}\right)^{12} - \left(\frac{\sigma}{r}\right)^{6} \right]$$

and Buckingham

$$U(r) = Ae^{-r\rho} - \frac{C}{r^6}$$

form for the potentials with parameters taken for the methylammonium (MA) molecules, $Pb^{2+}$ and $I^-$ ions from **Ref.** (*1*). Lennard-Jones and Buckingham potentials were truncated and shifted at 10 Å, and long ranged electrostatics were computed with PPPM/Ewald. For simulations with $Br^-$ or $Cl^-$, we derive parameters from the $I^-$ interactions by scaling the size and in proportion to the ratio of the known ionic radii and used geometric mixing rules as proposed by **Ref.** (*2*). Table S1 summarizes the parameters used where $H_1$ refers to those hydrogens attached to the nitrogen and $H_2$ to those hydrogens attached to the carbon.

Simulation protocol

Simulations are run to sample an ensemble with constant temperature, $T$, pressure, $p$, and chemical potential difference between two halide species, $\Delta\mu$. Constant temperature and pressure constraints are sampled using a Nose Hoover integrator with Parrinello-Rahman barostat (*3*) with 3 chains and 2 ps time constants suitable for a periodic system, and with the MA molecules held rigid following Zhang and Glotzer (*4*). Grand canonical Monte Carlo moves are added on top of the molecular dynamics to sample different halide compositions, or to sample different configurations at fixed composition, with 500 trial particle swaps every 200 integration steps. In this way, properties dependent on various average compositions as well as the susceptibility to changes in concentration, can be probed. A time step of 2 fs was used and most sets of calculations were equilibrated for 50 ps, with initial geometries take from (*5*) and 10 ns were used to converge averages. Integration and force evaluation were accomplished with LAMMPS (*6*).

*Table S1a: Buckingham potential parameters*

| Pair | A (kcal/mol) | $\rho$ (Å) | C (Å$^6$ kcal/mol) | Pair | A (kcal/mol) | $\rho$ (Å) | C (Å$^6$ kcal/mol) |
|---|---|---|---|---|---|---|---|
| Pb-Pb | 70359906 | 0.131258 | 0 | I-C | 112936 | 0.342426 | 0 |
| Pb-I | 103496 | 0.321737 | 0 | I-N | 112936 | 0.342426 | 0 |
| Pb-Br | 103496 | 0.30368 | 0 | Br-Br | 22793 | 0.42961 | 696.9495 |
| Pb-Cl | 103496 | 0.2917 | 0 | Br-Cl | 22793 | 0.4126616 | 696.9495 |
| Pb-C | 32690390 | 0.150947 | 0 | Br-C | 112936 | 0.323208 | 0 |
| Pb-N | 32690390 | 0.150947 | 0 | Br-N | 112936 | 0.323208 | 0 |
| I-I | 22793 | 0.482217 | 696.9495 | Cl-Cl | 22793 | 0.3963 | 696.9495 |
| I-Br | 22793 | 0.45515 | 696.9495 | Cl-C | 112936 | 0.3104578 | 0 |
| I-Cl | 22793 | 0.437198 | 696.9495 | Cl-N | 112936 | 0.3104578 | 0 |

*Table S1b: Lennard Jones parameters*

| Pair | $\epsilon$ (kcal/mol) | $\sigma$ (Å) |
|---|---|---|
| Pb-$H_1$ | 0.0140 | 2.26454 |
| Pb-$H_2$ | 0.0140 | 2.70999 |
| I-$H_1$ | 0.574 | 2.75 |
| I-$H_2$ | 0.574 | 3.10 |
| Br-$H_1$ | 0.574 | 2.5957 |
| Br-$H_2$ | 0.574 | 2.9260 |
| Cl-$H_1$ | 0.574 | 2.4932 |
| Cl-$H_2$ | 0.574 | 2.8105 |
| C-$H_1$ | 0.0414 | 2.23440 |
| C-$H_2$ | 0.0414 | 2.6798 |
| N-$H_1$ | 0.0517 | 2.1595 |
| N-$H_2$ | 0.0517 | 1.069 |

*Table S1c: Partial Charges Used*

| Species | Pb | I/Br/Cl | C | N | $H_1$ | $H_2$ |
|---|---|---|---|---|---|---|
| q | 2.030000 | -1.130000 | 0.771000 | -1.100000 | 0.540000 | 0.023000 |

Model validation and calculations and decomposition of the enthalpy of mixing

Using the model and simulation protocol described above, we have validated our model by computing the bulk lattice and elastic constants. Bulk moduli were computed for pure halide lattices by computing the compressibility from the mean squared volume fluctuations. This yielded 17.5, 17.4 and 15.4 GPa, for pure I, Br and Cl lattices. These are within 25% of experiment (*17*). In addition, we have computed average lattices constants of 6.26 Å, 5.80 Å and 5.50 Å for pure I, Br and Cl lattices which are within 1% agreement with experiment (*18*). Lattice constants as a function of composition are shown in Fig. S**1** with linear interpolations between pure lattices.

Results for the average concentration as a function of chemical potential difference are shown in Fig. S**1**. A reference value of 5.5 kcal/mol and 20 kcal/mol is used to place both curves on the same scale. These curves indicate that exchange between $I^-$ and $Br^-$ is continuous, though with a peak in susceptibility around $\Delta\mu=0$. This is consistent with the ground state stability of these mixtures. However, exchange between $I^-$ and $Cl^-$ appears discontinuous, with a jump in concentration around $\Delta\mu=0$, consistent with the observed instability of mixtures of these materials.

In order to understand the energetic driving forces for phase separation we have computed the enthalpy of mixing at fixed composition and either at fixed stress, 1 bar, or at fixed volume. We follow the procedure outlined above for the molecular dynamics simulations, and compute the enthalpy per unit cell as

$$\Delta H_{\mathrm{mix}}(x) = \langle H \rangle - x[\langle H(x=0) \rangle - \langle H(x=1) \rangle$$

where *x* is the composition of the smaller halide in each mixture. The constant volume calculations are done with a volume fixed by linearly interpolating between the pure lattices. The results of these calculations are shown in Fig. **S2** where the red data denotes constant strain and the blue constant stress. The shaded regions in those plots are fits to the Flory form,

$$\Delta H_{\mathrm{mix}}(x) = \chi x(1-x)$$

which allows us to extract a critical demixing temperature, assuming a Flory-Huggins form for the free energy.

Extension to PIMD simulations and free energy calculations

To extend the molecular model to incorporate effects from photo-generated charges, we used a path integral molecular dynamics description on an excess charge following Refs (*7*, *8*), with pseudo potentials following Ref (*9*). The form of the pseudo potential consisted of simple Coulomb interactions for the excess electron and anionic species, and short-ranged truncated Coulomb interactions for the cations. The cut-off radii were chosen as the ionic radii of each species and reasonably recover the known ionization potentials for each cation. The values are summarized in Table S2. Ring polymers with 1024 beads were found to be sufficient to converge the average radius of gyration, and a fictitious mass of 1 amu was used in the calculations with a timestep of 0.5 fs.

*Table S2: Short range cutoffs*

| Species | Pb | C | $H_1$ | $H_2$ |
|---|---|---|---|---|
| R/Å | 3.1 | 1.1 | 1.0 | 1.0 |

Simulations with the excess charge were accomplished using the same procedure outlined above. To compute the free energies as a function of composition, simulations were run with $\beta\Delta\mu$ = {-3,3}, in steps of 0.5. In the case of the excess charge, where nucleation barriers between iodide-rich and bromide-rich phases result in poor sampling near coexistence, replica exchange was performed by scaling the temperature associated with grand-canonical moves between 300 K-600 K in increments of 30 K. WHAM was used to combine the different ensemble calculations into a single free energy estimate (*10*), reweighted to coexistence, with errors computed from standard bootstrapping. The binding energy is computed from the change in the average potential energy and the deformation size is computed from the radius of gyration of the ring polymer weighted by the electron phonon coupling.

Landau theory with strain and excess charge

We start by assuming that the phase separation between different halide species satisfies a Flory-Huggins solution theory,

$$H_{\mathrm{c}} = \int_{\mathbf{r}} \chi\phi(\mathbf{r})[1-\phi(\mathbf{r})] + T\{\phi(\mathbf{r})\ln[\phi(\mathbf{r})] + [1-\phi(\mathbf{r})]\ln[1-\phi(\mathbf{r})]\}$$

where $\chi$ is related to the excess enthalpy of mixing, $T$ is the temperature, and $\phi$ is the local concentration of iodide relative to bromide. Assuming that the light does not induce plastic deformations or other large scale morphological transitions the strain field can be assumed to be Gaussian,

$$H_{\mathrm{l}} = \int_{\mathbf{r}} \mathbf{K}\,\mathbf{\Sigma}^2(\mathbf{r})/2(1-\nu)$$

Here $\Sigma$ is the local strain field, $K$ is bulk modulus in the mixed phase and $\nu$ is Poisson's ratio. For simplicity the elasticity is assumed to be isotropic. To lowest order these fields are coupled with a bilinear term,

$$H_{\mathrm{c,l}} = \int_{\mathbf{r}} c_2 \mathbf{\Sigma}(\mathbf{r})\phi(\mathbf{r})$$

where the coupling coefficient $c_2$ is taken to be proportional to the change in lattice constants, $a$, with composition (*11*):

$$c_2 = 2\eta K/(1-\nu)$$

where $\eta = d \ln a/d\phi$ evaluated at $\phi=1/2$. This theory offers a complete description of the ground state free energy surface. Adding these three terms together, integrating out the strain fields and expanding $\phi$ around 0.5, a $\phi^4$ theory is obtained (*12*),

$$H = \int_{\mathbf{r}} m[\phi(\mathbf{r}) - 1/2]^2 + u[\phi(\mathbf{r}) - 1/2]^4$$

where $m=2T-\chi-2K\eta^2/(1-\nu)$, and $u=4T/3$. The free energy is determined by evaluating this hamiltonian within mean field theory by finding solutions to the equation,

$$\frac{dH}{d\bar{\phi}(r)} = 0$$

that minimize the Hamiltonian. Then the per unit cell free energy is

$$\Delta F(x) = H[\bar{\phi}].$$

For Br/I mixtures, *m is* taken from the molecular dynamics simulations and set to $m=2T(K)-390K$.

In order to describe light-induced phase separation an additional term reflecting the electronic degrees of freedom must be added. We do this following the deformation potential theory for electron-phonon interactions (*13*), and make a semiclassical appromixation to decouple the electronic and ionic motions (*14*). Specifically we add the lowest order coupling between excess charge density and the strain and composition fields,

$$H_{\mathrm{e,l-c}} = \int_{\mathbf{r}} \alpha \mathbf{\Sigma}(\mathbf{r})|\Psi(\mathbf{r})|^2 + \epsilon\phi(\mathbf{r})|\Psi(\mathbf{r})|^2$$

where $\alpha$ is the dimensionless electron-phonon coupling constant and $\epsilon<0$ is the energetic bias of an excess charge to reside on the Iodide rich regions. $|\Psi|^2$ is the excess charge density localized to a region $l^3$. The kinetic energy of the electrons has been neglected. This additional term in the Hamiltonian is linear and permits the strain field from still being integrated out. This results in an effective hamiltonian in the excited state along the symmetry line $\epsilon=0$,

$$H = \int_{\mathbf{r}} m[\phi(\mathbf{r}) - 1/2]^2 + u[\phi(\mathbf{r}) - 1/2]^4 - g|\Psi(\mathbf{r})|^2|\phi(\mathbf{r}) - 1/2$$

where $g = 2\alpha|\eta|$. The mean field approximation can be used to compute the free energy, phase diagram and extent of demixing as done previously in the ground state. For the calculation in Fig 2 of the main text, we use $g = 0.57\,K$, which is arrived at from the polaron binding energy and extent computed from molecular dynamics simulations.

Discretizing the theory to study clustering dynamics

In order to simulate the clustering process, we develop an effective discretized version of

the Landau theory outlined above. We do this by making two approximations 1) that the phase separation can be modeled by an Ising model and 2) that the influence of the polaron is to locally renormalize the coupling between the nearest neighbor sites. The hamiltonian for the model is

$$\mathcal{H} = -\sum_{<ij>} J_{ij} s_i s_j - \lambda \int_r \sum_i \rho(r) s_i \delta(r - r_i)$$

where the sum runs to the *N* sites, $s_i = \{\pm 1\}$, $\delta(x)$ is Dirac's delta function, and $\boldsymbol{\rho(r)}$ is the polaron density parameterized by a center and a length, *l*. The density is assumed to have the form

$$\rho(\vec{r}) = \left(\frac{1}{2\pi\ell}\right)^{3/2} e^{-\vec{r}^2/2\ell^2}$$

and the local coupling depends on its location through

$$J_{i,j} = J_o + \Delta \int_r \sum_{i,j} \rho(r) \delta(r - r_{ij})$$

where $\lambda$ biases the polaron to be in the iodide rich regions.

We associated nearest neighbor swapping between lattice sites to model the diffusion of the halides, and a continuum diffusive dynamics of the excess charge. The characteristic timescales for both of these motions is known experimentally, with halide hopping occurring every 1 ms (*15*), and polaron motilities about 1000x faster (*16*). The dynamics are propagated with Monte Carlo using standard Metropolis acceptance criteria with the hamiltonian above.

The parameters used to reproduce the PL intensity as a function of time in Fig. 3B are, $T=1$, $J_o=0.3$, $\lambda=0.2$, $l=5$, $\Delta=0.5$ with *N* swap attempts set to a physical time of 1 ms. The system is simulated on circle of radius 50 sites with open boundary conditions. These conditions mimic the strain relaxation at the boundary of the grain, effectively biasing the minority species to the boundary in the demixed phase. To simulate the PL intensity as a function of time, the system is initialized with a uniform spin distribution and the polaron placed in the center of the grain. To converge Fig 3B, 10,000 trajectories were averaged.

**Supplementary Text**

Electron beam exposure does not cause demixing

The electron beam excitation does not cause demixing due to the mode of excitation. As the electron beam scans across the sample, the beam dwells on each pixel for ~20 μs before moving to the next pixel. Therefore, excitations are present at each pixel for ~20 μs plus the lifetime of the charge carriers, which is much shorter than the dwell time. According to Figure 3B, this is not nearly enough time to induce cluster formation, which would require the constant replenishing of carriers during steady state (seconds to minutes) illumination.

## Supplementary Figures

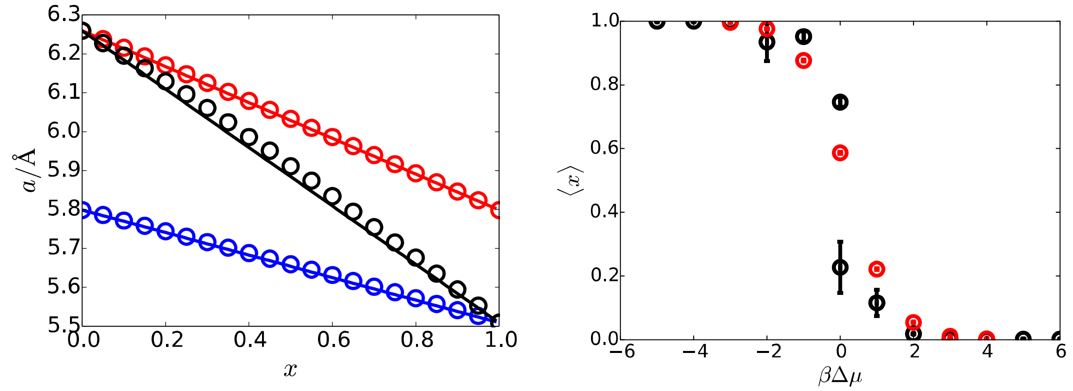


**Fig. S1.** Model validation calculations. (left) Lattice constants as a function of composition for mixtures of $Br_xI_{1-x}$ (red), $I_xCl_{1-x}$ (black), and $Br_xCl_{1-x}$ (blue). (right) Average composition at constant chemical potential difference for mixtures of $Br_xI_{1-x}$ (red), $I_xCl_{1-x}$ (black) While ‹*x*› changes continuously through $\Delta\mu$=0 for $Br_xI_{1-x}$ mixtures, the abrupt change for $I_xCl_{1-x}$ mixtures reflects its room temperature instability.

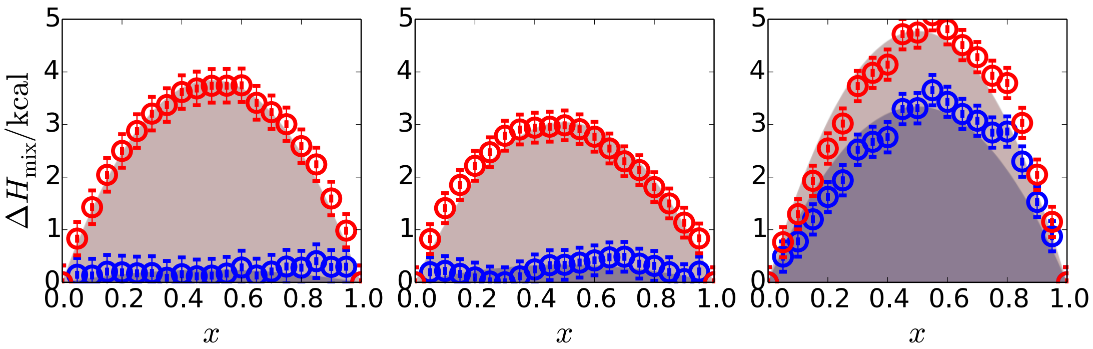


**Fig. S2.** Excess enthalpies of mixing computed at constant volume (red) or constant stress (blue) for mixtures of (left) $Br_xI_{1-x}$, (middle) $Br_xCl_{1-x}$, and (right) $I_xCl_{1-x}$.

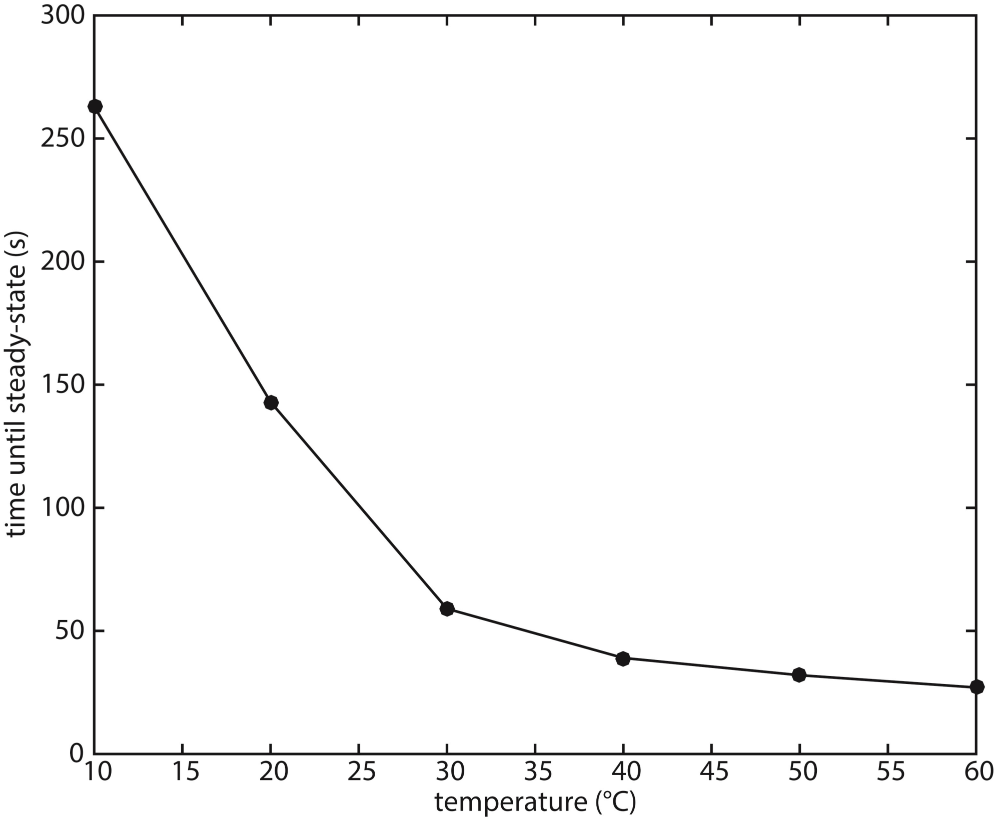


**Fig. S3. Probing the temperature dependence of phase separation with PL.** The time it takes for the PL peak of the iodide-rich clusters to reach a maximum value for a $MAPb(Br_{0.1}I_{0.9})_3$ film at 100 $mW/cm^2$ as a function of temperature with a 405 nm excitation source.

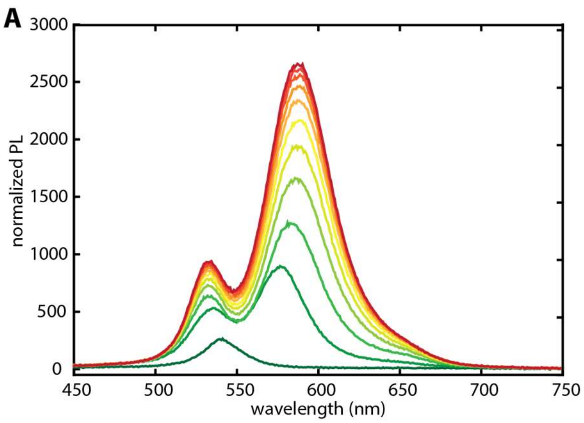


**Fig. S4. PL of $CsPb(Br_{0.1}I_{0.9})_3$.** (**A**) PL spectra of $CsPb(Br_{0.1}I_{0.9})_3$ collected every 1 min at 100 mW/cm$^2$. (**B**) Normalized PL intensity versus time of the iodide cluster peak. The wavelength shift of the iodide cluster PL peak here is much less significant than that of $MAPb(Br_{0.1}I_{0.9})_3$. Furthermore, compared to the normalized PL versus time plot of $MAPb(Br_{0.1}I_{0.9})_3$ (Figure 3B), the normalized PL plot of $CsPb(Br_{0.1}I_{0.9})_3$ shows that it takes much longer for the iodide cluster peak to saturate.

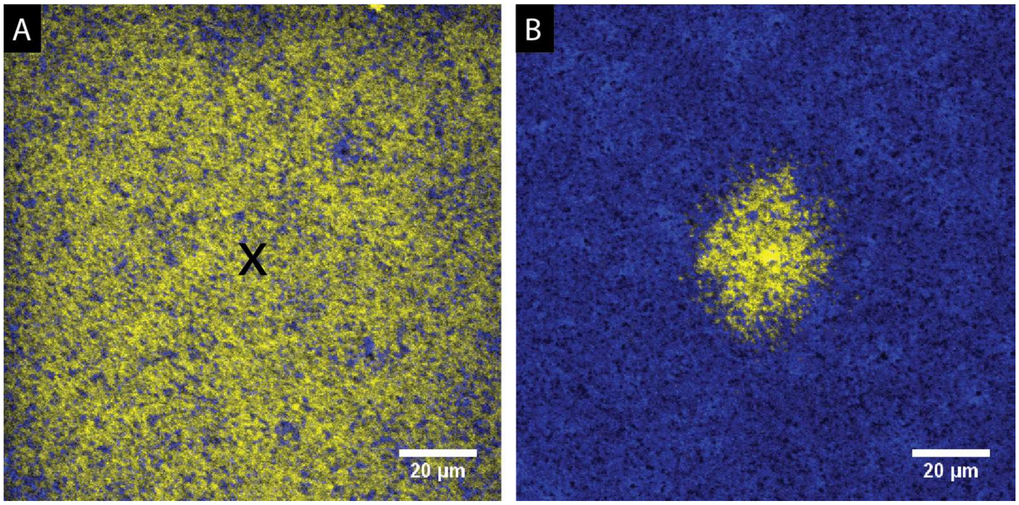


**Fig. S5. Demonstration that red light can stabilize iodide-rich clusters.** (**A**) Confocal microscopy image of a $CH_3NH_3Pb(I_{0.1}Br_{0.9})_3$ film after light soaking with 405 nm light for 5 minutes. Emission from Br-rich regions (500-550 nm, blue) and I-rich regions (650-750 nm, yellow) are recorded simultaneously. After 5 min, the 405 nm light is turned off and a 635 nm laser is focused on the X. (**B**) After 5 min, an image is recorded with 405 nm excitation. The spot in the middle of the image still emits at 690 nm, confirming that clusters are stabilized by 635 nm light.

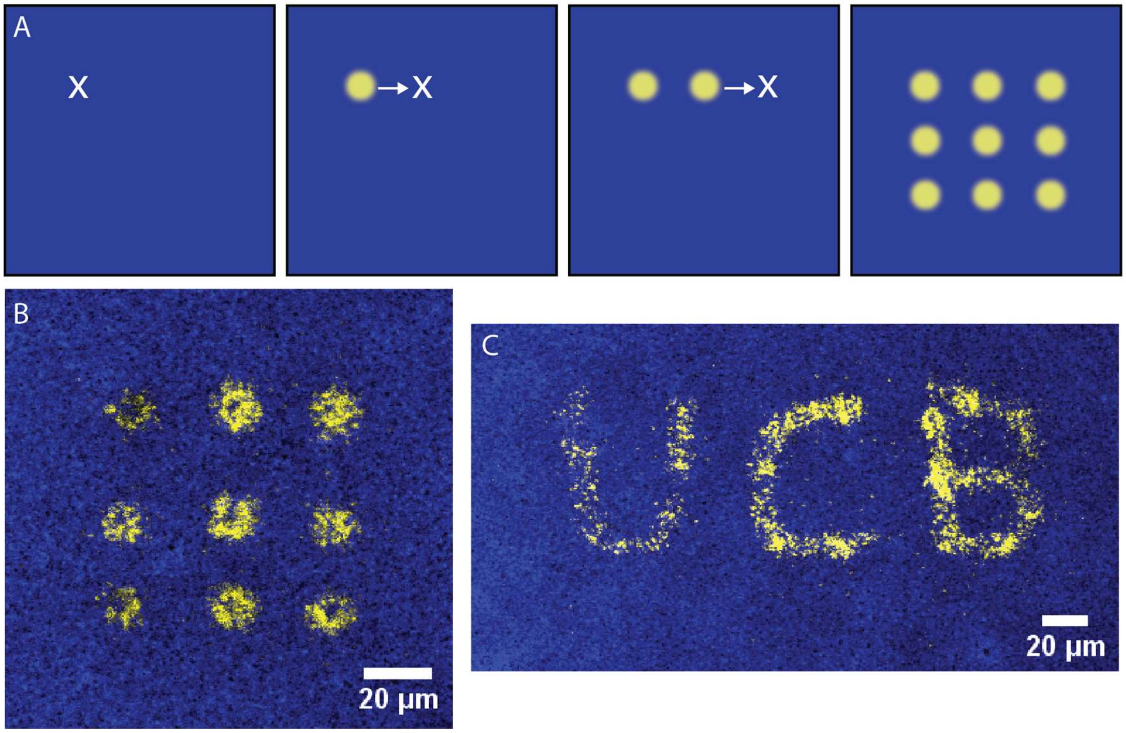


**Fig. S6. Transiently patterning mixed halide perovskite films.** (**A**) Schematic of the series of steps used to generate a pattern in a $CH_3NH_3Pb(I_{0.1}Br_{0.9})_3$ film. I-rich areas are yellow and Br-rich areas are blue. To experimentally achieve this scheme a 660 nm LED illuminates the sample continuously to stabilize any clusters formed with a focused 405 nm laser (white X). This 405 nm laser is scanned to different points to form a 3x3 grid pattern by inducing phase separation at discrete locations. An array of spots (**B**) and an image of 'UCB' (**C**) provide experimental realizations of the scheme, imaged (also using 405 nm excitation) after cluster patterning.

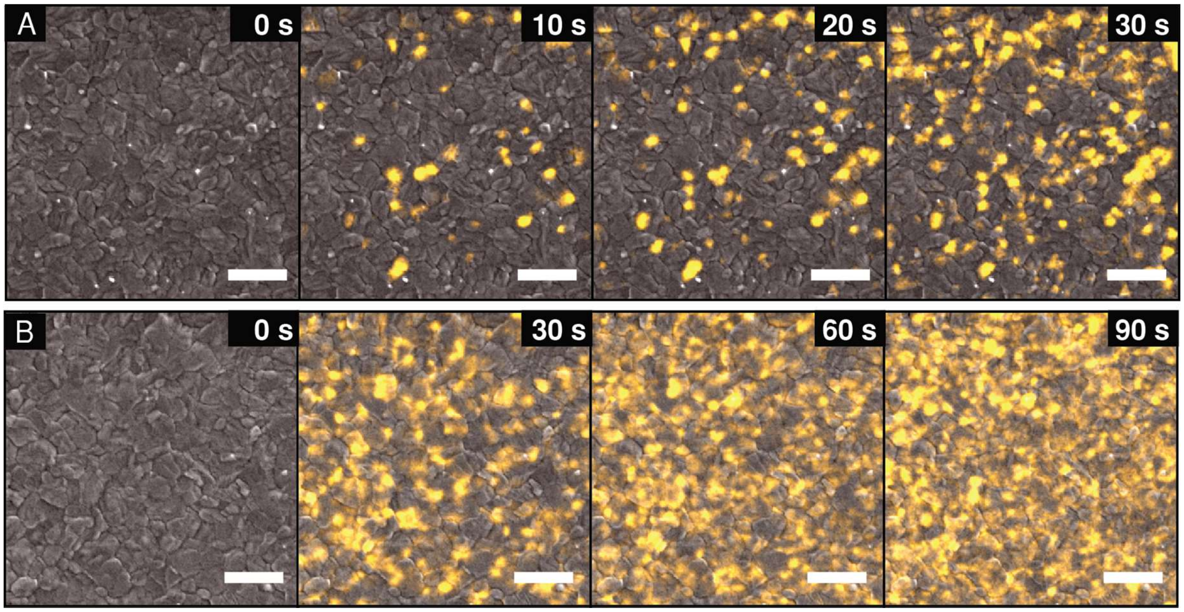


**Fig. S7. CL images of I-rich cluster formation at 1100 mW/cm$^2$.** At higher illumination intensity the rate of cluster formation increases because of the increase in number of photogenerated carriers capable of intercepting iodide concentration fluctuations. (**A**) Light soaking for 10 s between CL scans. (**B**) Light soaking for 30 s between CL scans. The scale bars are 2 μm.

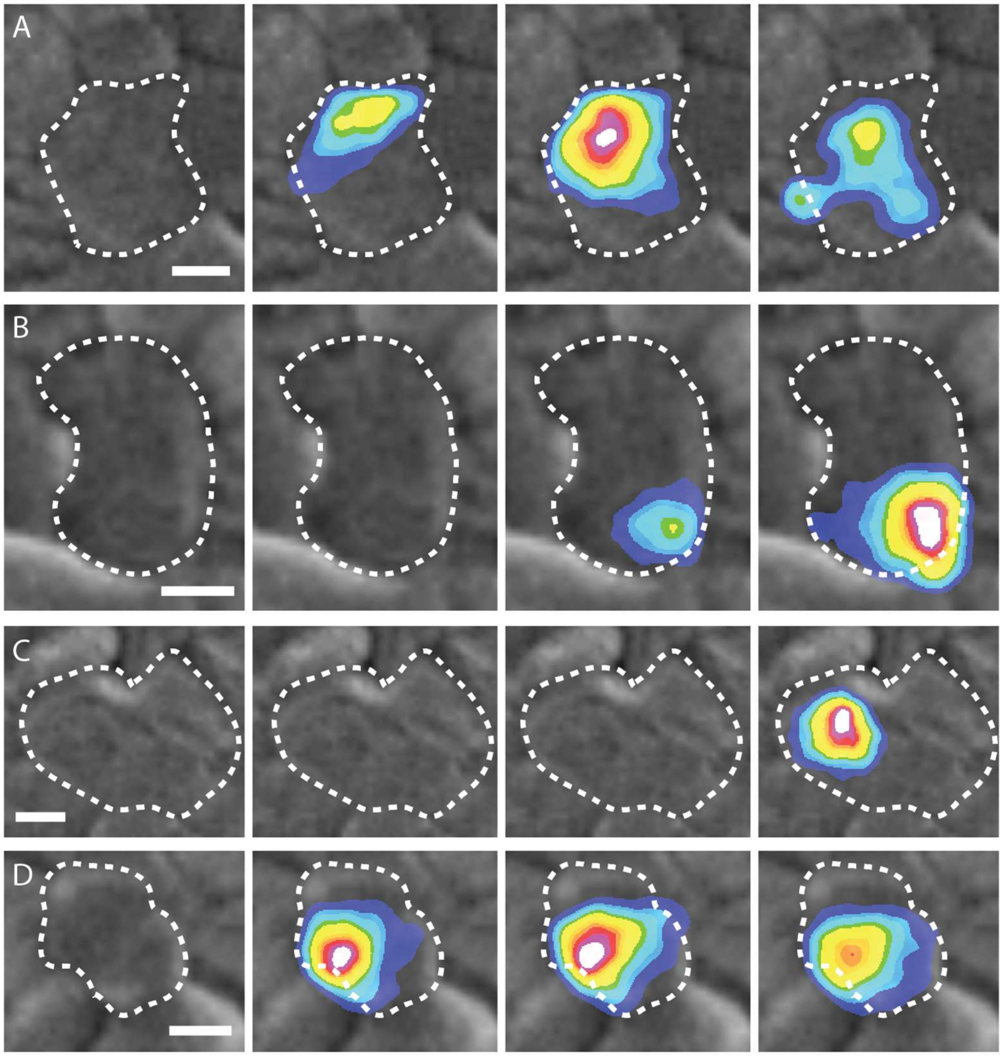


**Fig. S8. Additional CL data of the formation of iodide-rich clusters.** (**A-D**) Examples of other cluster formation in single domains with 10 seconds of light soaking in between frames. The scale bars are 300 nm.

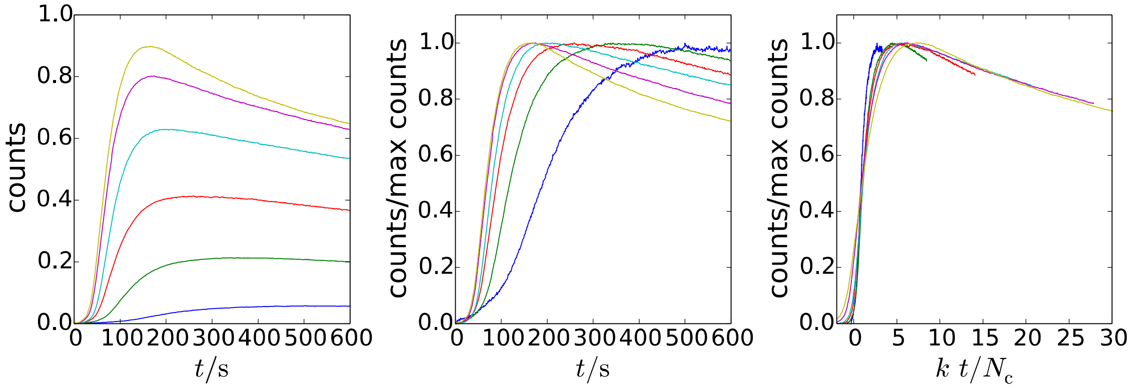


**Fig. S9. Time dependence of the experimental PL intensity at different illumination intensities.** (left) Time dependence of the integrated PL intensity between 600-800 nm for excitation intensities of 4.0, 10, 18, 25, 35, 45, and 55 mW/cm$^2$. (middle) PL intensity versus time, normalized by respective maxima. (right) PL intensity, normalized by its maximum, versus time scaled by the inverse carrier concentration. The trends in maximum PL intensity and in time for it to be achieved are analyzed in Figures S11 and S10, respectively.

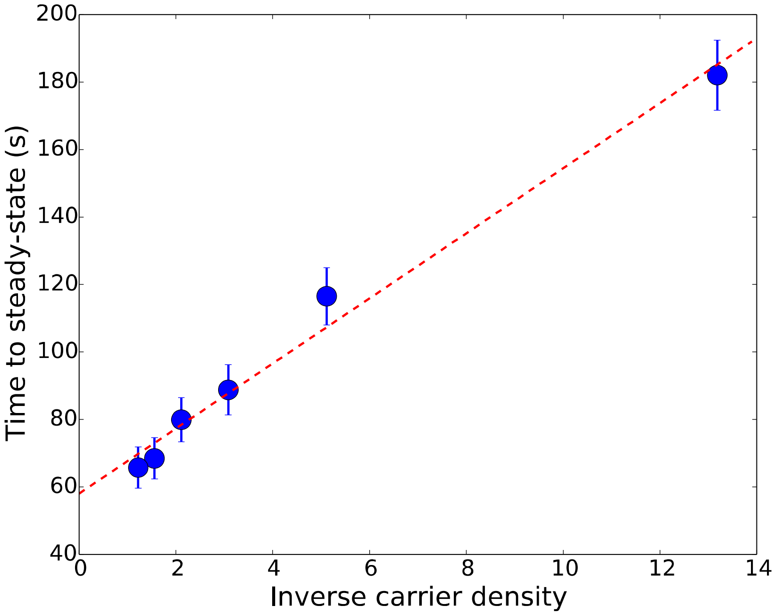


**Fig. S10. Time to steady state scales linearly with inverse carrier density.** An average time to steady state as a function of inverse charge carrier density. The average time is computed by fitting the PL intensity versus time in Fig. S9 to a functional form, $\mathcal{I}(t) = A \tanh((t-\tau)/\delta\tau) + Bt + C$, where $\tau$ is taken to be the mean time to steady state and $\delta\tau^{1/2}$ is used as the error.

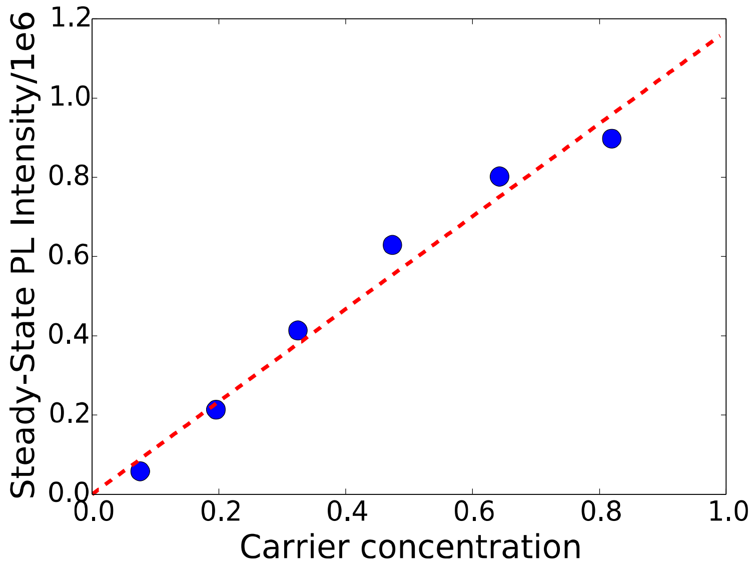


**Fig. S11. Steady state amount of iodide-rich composition is proportional to carrier concentration.** Maximum PL intensity from Fig. S9 as a function of carrier concentration. Assuming each cluster is equally luminescent, and that the clusters are spherical on average, the linear relationship allows us to extract a mean cluster size referenced in the main text.

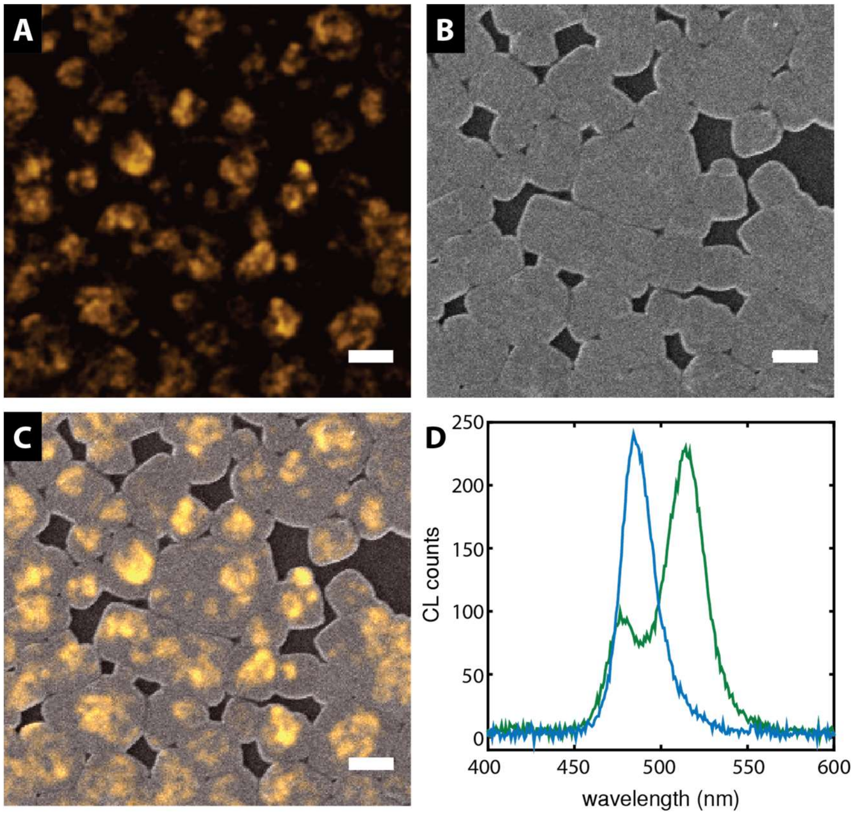


**Fig. S12. Light-induced halide phase separation in a $MAPb(Br_{0.5}Cl_{0.5})_3$ film.** (**A**) CL image (509 nm longpass filter), (**B**) SE image, and (**C**) CL/SE overlay of a $MAPb(Br_{0.5}Cl_{0.5})_3$ film after 1 min light soaking at 100 mW/cm$^2$. Scale bars are 1.0 µm. (**D**) CL spectra before (blue) and after (green) light soaking.

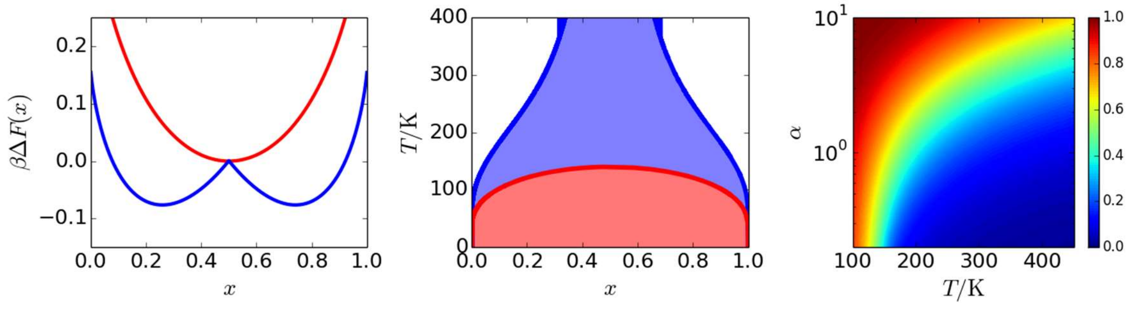


**Fig. S13. Free energies and phase behavior for Br/Cl mixtures.** Using $m$ = 2T(K)-280K, as computed from the molecular dynamics simulations, and the same $g$ used in the Br/I case, we construct the free energies, phase diagrams and extents of demixing for solid solutions of Br/Cl. (left) Free energy per unit cell computed from mean field theory in the ground (red) and photo-excited (blue) states. (middle) Phase diagram in the ground (red) and excited (blue) states. (right) Extent of demixing as a function of electron-phonon coupling.

## Supplementary Movie Captions

**Movie S1. Molecular dynamics simulation of a 99% isosurface of excess charge density on the perovskite lattice.**

**Movie S2. Sequence of CL images of phase separation with 10 s light soaking intervals at 50 mW/cm$^2$.** Movie of the CL images shown in Figure 3A.

**Movie S3. Sequence of CL images of phase separation with 30 s light soaking intervals at 50 mW/cm$^2$.** Movie of the CL images shown in Figure 3B.

**Movie S4. Sequence of CL images of phase separation with 10 s light soaking intervals at 1100 mW/cm$^2$.** Movie of the CL images shown in Figure S7A.

**Movie S5. Sequence of CL images of phase separation with 30 s light soaking intervals at 1100 mW/cm$^2$.** Movie of the CL images shown in Figure S7B.

**Movie S6. Cluster formation simulation.** Movie of a cluster formation simulation with iodide-rich regions in yellow and bromide-rich regions in blue.

## Supplementary References

1. A. Mattoni, A. Filippetti, M. I. Saba, P. Delugas, Methylammonium Rotational Dynamics in Lead Halide Perovskite by Classical Molecular Dynamics: The Role of Temperature. *J. Phys. Chem. C.* **119**, 17421–17428 (2015).

2. G. V. Lewis, C. R. A. Catlow, Potential models for ionic oxides. *J. Phys. C Solid State Phys.* **18**, 1149 (1985).

3. M. Parrinello, A. Rahman, Polymorphic transitions in single crystals: A new molecular dynamics method. *J. Appl. Phys.* **52**, 7182–7190 (1981).

4. Zhang, S. C. Glotzer, Self-Assembly of Patchy Particles. *Nano Lett.* **4**, 1407–1413 (2004).

5. H. Mashiyama, Y. Kurihara, T. Azetsu, Disordered cubic perovskite structure of CH3NH3PbX3 (X=Cl, Br, I). *J.- Korean Phys. Soc.* **32**, S156–S158 (1998).

6. S. Plimpton, Fast Parallel Algorithms for Short-Range Molecular Dynamics. *J. Comput. Phys.* **117**, 1–19 (1995).

7. D. Chandler, P. G. Wolynes, Exploiting the isomorphism between quantum theory and classical statistical mechanics of polyatomic fluids. *J. Chem. Phys.* **74**, 4078–4095 (1981).

8. D. Chandler, Y. Singh, D. M. Richardson, Excess electrons in simple fluids. I. General equilibrium theory for classical hard sphere solvents. *J. Chem. Phys.* **81**, 1975–1982 (1984).

9. M. Parrinello, A. Rahman, Study of an F center in molten KCl. *J. Chem. Phys.* **80**, 860–867 (1984).

10. S. Kumar, J. M. Rosenberg, D. Bouzida, R. H. Swendsen, P. A. Kollman, THE weighted histogram analysis method for free-energy calculations on biomolecules. I. The method. *J. Comput. Chem.* **13**, 1011–1021 (1992).

11. J. W. Cahn, On spinodal decomposition. *Acta Metall.* **9**, 795–801 (1961).

12. P. M. Chaikin, T. C. Lubensky, *Principles of Condensed Matter Physics* (Cambridge University Press, Cambridge; New York, NY, USA, 2000).

13. G. Whitfield, P. B. Shaw, Interaction of electrons with acoustic phonons via the deformation potential in one dimension. *Phys. Rev. B*. **14**, 3346–3355 (1976).

14. G. Kalosakas, S. Aubry, G. P. Tsironis, Polaron solutions and normal-mode analysis in the semiclassical Holstein model. *Phys. Rev. B*. **58**, 3094–3104 (1998).

15. C. Eames *et al.*, Ionic transport in hybrid lead iodide perovskite solar cells. *Nat. Commun.* **6**, 7497 (2015).

16. S. D. Stranks *et al.*, Electron-Hole Diffusion Lengths Exceeding 1 Micrometer in an Organometal Trihalide Perovskite Absorber. *Science*. **342**, 341–344 (2013).

17. Y. Rakita, S. R. Cohen, N. K. Kedem, G. Hodes, D. Cahen, Mechanical properties of APbX 3 (A = Cs or CH3NH3; X = I or Br) perovskite single crystals. *MRS Commun.* **5**, 623–629 (2015).

18. A. Poglitsch, D. Weber, Dynamic disorder in methylammoniumtrihalogenoplumbates (II) observed by millimeter-wave spectroscopy. *J. Chem. Phys.* **87**, 6373–6378 (1987).
